# Supplementary material for: Autoregressive Density Modeling with the Gaussian Process Mixture Transition Distribution
Source: arXiv:2007.09279 source file (2020-07-17)
Supplement: Supplementary file 1 [file appendix_skew.tex]

\newpage

\section{Mixture components with long tails and skew}
\label{sec:appendix_skew}

The intercept component in (\ref{eq:gpmtd1}) is instrumental for the Old Faithful example in that it provides a vehicle both for bimodality (when $y_{t-1} > 70$ minutes) and a pair of outliers (at $y_{t-1} \approx 70$ minutes). As noted in Section \ref{sec:intro}, \citet{le1996gmtd} also use an independent component for outliers. If, however, certain characteristics of the transition distribution systematically associate with a certain lag, it is more appropriate to accommodate them in the corresponding mixture component. Adding flexibility to the mixture component distributions further helps disentangle two model objectives: transition density estimation through mixtures and lag selection. If the mixture is used primarily for lag selection, our method relates to \citet{hansen1994ARdensity}, who explores using parametric extensions of Gaussian transition densities. In this section, we apply two standard extensions aimed at increasing flexibility without sacrificing parsimony or computational convenience.

We first consider allowing long-tailed component distributions. Using the student $t$ distribution's well-known representation as a scale mixture of Gaussian distributions, we introduce independent latent variables $\{ \varphi_{\ell,t} \}$, associated with each component and observation, and distributed gamma with shape $\eta_\ell/2$ and rate $\eta_\ell/2$. The variance of each component in the first line of (\ref{eq:hier}) becomes $\sigma_\ell^2 / \varphi_{\ell,t}$. We complete the specification with independent gamma priors for $\eta_\ell - 2$, for $\ell = 0, \ldots, L$, ensuring two finite moments in the mixture components. This extension preserves Gaussianity of full conditional updates in the Gibbs sampler with the following minor changes. The identity matrices that appear in $\bm{W}$ and in $\bm{\Sigma}$ in Step 4 of the component-specific Gibbs scan in Appendix \ref{sec:appendix_mixcomp_updates}
are replaced with $\diag(\varphi_{\ell, t_{i1}}^{-1}, \ldots, \varphi_{\ell, t_{in_\ell}}^{-1})$. A fifth and sixth step are added to the Gibbs scan to update each $\varphi_{t,\ell}$ (conditionally conjugate gamma) and $\eta_\ell$ (non-conjugate, updated with Metropolis or with a discrete prior). Steps 1, 3, and 4 of the full Gibbs sampler in Appendix \ref{sec:appendix_MCMC} likewise reflect observation-specific variance scaling by $\{\varphi_{\ell, t}\}$, but retain their basic forms.

We next admit skewness in addition to long tails. We employ the scale mixture of skew-normal distributions of \citet{cancho2011skew}, who develop a framework for Bayesian inference in nonlinear regression with skewed and/or long-tailed errors. The skew-normal distribution derives from the construction of \citet{azzalini1985skew}. Random variable $Y$ is said to follow the skew-normal distribution if it has density
\begin{align}
    \label{eq:skewnormaldens}
    \phi(y \mid \mu, \sigma^2, \xi) = 2 \phi \left( \frac{ y - \mu }{ \sigma }  \right) \Phi \left( \xi \frac{ y - \mu }{ \sigma }  \right) \, ,
\end{align}
where $\phi(\cdot)$ is the standard Gaussian density function, $\Phi(\cdot)$ is the standard Gaussian cumulative distribution function, and the parameter $\xi \in \mathbb{R}$ influences skewness. A stochastic representation for $Y$ \citep{henze1986skew} facilitates modeling with the skew-normal distribution, for which significant development in the last few decades includes both nonlinear regression and mixture models \citep{lin2007skewmix}.

\citet{cancho2011skew} induce a scale mixture by including a latent positive-valued random variable $\varphi$, which for our purposes will have the same gamma distribution introduced above, and replacing all instances of $\sigma$ in (\ref{eq:skewnormaldens}) with $\sigma / \sqrt{\varphi}$. Integrating (\ref{eq:skewnormaldens}) with respect to the density of $\varphi$ produces the scale mixture of skew normal distributions, which in our case is a skew-$t$ with $\eta$ degrees of freedom. They report the stochastic representation as $ Y = \mu + \Delta V + \sqrt{\tau / \varphi} \, V_1$, where $\Delta = \sigma \, \delta$ with $\delta = \xi / \sqrt{ 1 + \xi^2 }$, $\tau = \sigma^2 (1 - \delta^2)$, $V = \lvert V_0 \rvert / \sqrt{\varphi}$, and $V_0$ and $V_1$ are independent standard Gaussian random variables. Setting $\xi=0$ results in a scale mixture of normal distributions, while fixing $\varphi=1$ produces skew only. This parameterization yields conditional conjugacy and thus convenient posterior sampling if we specify independent Gaussian and inverse-gamma priors for $\Delta$ and $\tau$, respectively.

Conditional on allocation membership $z_t=\ell$, which we omit from the 
notation for simplicity, the modified contribution of $y_t$ to the GPMTD is given in generative order as
\begin{align}
    \label{eq:skewnormalhier}
    \varphi_t \mid \eta & \sim \Gammadist \left( \eta/2, \eta/2 \right) \, , \nonumber \\
    p( V_t \mid \varphi_t, \eta ) & \propto \Ndist \left( V_t \mid b_v, \varphi_t^{-1} \right) 1_{(V_t > b_v)} \, , \\
    y_t \mid V_t, \varphi_t, \mu, f, \sigma^2, \eta & \sim \Ndist \left( \mu + f(x_{t,\ell}) + \Delta V , \tau / \varphi \right) \, , \nonumber
\end{align}
where $b_v = -\sqrt{\eta/\pi} \, \Gamma \left( [\eta - 1]/2 \right) / \Gamma \left( \eta / 2  \right) $. The shift by $b_v$ ensures that the component has mean $\mu + f(x_{t,\ell})$ \citep{cancho2011skew}. Note that the $(\varphi_t, V_t, \mu, f, \Delta, \tau, \eta)_\ell$ tuple is specific to mixture component $\ell$. This setup admits a sampling scheme similar to that given in Appendix \ref{sec:appendix_mixcomp_updates}, in which matrix $\bm{W}$ again includes $ \{ \varphi_t \} $ and $\bm{1} \mu$ is replaced with a linear regression form in which $\{ V_t \}$ populates the second column of a design matrix with coefficient vector $(\mu, \Delta)$. The full conditional distributions for $\varphi_t$ and $V_t$ are gamma and truncated normal, respectively \citep{cancho2011skew}. Because $\sigma^2$ is coupled with other parameters, the Gaussian process variance $\kappa \, \sigma^2$ is replaced with a single, unrelated variance parameter.
